# Supplementary material for: Multilinear Dirichlet Processes
Source: arXiv:2106.08852 source file (2021-06-16)
Supplement: Supplementary file 1 [file appendix.tex]

\section{Computation}

\subsection{Update $\mat{U}$}
Encode the value of $b_m^{j_1,\dots,j_N}$ using a vector $ \vect{z}_m^{j_1,\dots,j_N} \in \reals^{I_1 \times I_2 \times \cdots \times I_N}$, where the $i_1,\dots,i_N$th element of $ \vect{z}_m^{j_1,\dots,j_N} $ is $1$ if $b_m^{j_1,\dots,j_N} = i_1,\dots,i_N$. For the following derivation, we use $\vect{z}$ by omitting the superscript and subscript of $\vect{z}_m^{j_1,\dots,j_N}$ for clarity.
\begin{align}
\mathcal{J}_{-n} = \{j_1,\dots,j_{n-1},j_{n+1},\dots, j_N\} \nonumber \\
\mathcal{I}_{-n} = \{i_1,\dots,i_{n-1},i_{n+1},\dots, i_N\} \nonumber \\
p(b_m^{j_1,\dots,j_N} = i_1,\dots,i_N| \mat{U}) = \frac{e^{u_{i_1}^{1,j_1}u_{i_2}^{2,j_2}\dots u_{i_N}^{N,j_N}}}
{\sum\limits_{k_1,k_2,\dots,k_N}e^{u_{k_1}^{1,j_1}u_{k_2}^{2,j_2}\dots u_{k_N}^{N,j_N}}}  \nonumber \\
  =   \frac{e^{(\vect{u}^{1,j_1} \otimes \vect{u}^{2,j_2}\dots \otimes \vect{u}^{N,j_N})^T \times \vect{z}}}
{\sum\limits_{k_1,k_2,\dots,k_N}e^{u_{k_1}^{1,j_1}u_{k_2}^{1,j_2}\dots u_{k_N}^{N,j_N}}} \nonumber \\
L = \log{\prod\limits_{\mathcal{J}_{-n}}\prod\limits_{m=1}^{M^{j_1,\dots,j_N}}p(b_m^{j_1,\dots,j_N})} \nonumber \\
  = \sum\limits_{\mathcal{J}_{-n}}(\sum\limits_{m=1}^{M^{j_1,\dots,j_N}}(\vect{u}^{1,j_1} \otimes \vect{u}^{2,j_2}\dots \otimes \vect{u}^{N,j_N})^T \times \vect{z}- M^{j_1,\dots,j_N}\log{\sum\limits_{k_1,k_2,\dots,k_N} e^{u_{k_1}^{1,j_1}u_{k_2}^{2,j_2}\dots u_{k_N}^{N,j_N}}}) \nonumber \\
\frac{\partial L}{\partial {u}^{n,j_n}_{i_n}} = \sum\limits_{\mathcal{J}_{-n}}(\sum\limits_{m=1}^{M^{j_1,\dots,j_N}}(\vect{u}^{1,j_1} \otimes \dots \vect{u}^{n-1,j_{n-1}}\otimes\vect{u}^{n+1,j_{n+1}}\dots \otimes \vect{u}^{N,j_N})^T\times \tilde{\vect{z}} - \nonumber \\
\sum\limits_{\mathcal{K}_{-n}} u_{k_1}^{1,j_1}\dots u_{k_N}^{N,j_N} e^{u_{k_1}^{1,j_1}\dots u_{k_N}^{N,j_N} u^{n,j_n}_{i_n}-\log{\sum\limits_{k_1,k_2,\dots,k_N}e^{u_{k_1}^{1,j_1}u_{k_2}^{1,j_2}\dots u_{k_N}^{N,j_N}}}})
\end{align}

\begin{align}
p(b_s^{i,j,k}) = \frac{e^{\vect{v}^i \otimes \vect{w}^j \otimes \vect{u}^k \times \vect{z}_s^{i,j,k}}}{\sum\limits_{m,n,l} e ^{v^i_m w^j_n u^k_l}} \\
L = \log{\prod\limits_{i,j}\prod\limits_{s=1}^{M^{i,j,k}}p(b_s^{i,j,k})} \nonumber \\
  = \sum\limits_{i,j}(\sum\limits_{s=1}^{M^{i,j,k}}\vect{v}^i \otimes \vect{w}^j \otimes \vect{u}^k \times \vect{z}_s^{i,j,k}- M^{i,j,k}\log{\sum\limits_{m,n,l} e^{v^i_m w^j_n u^k_l}}) \nonumber \\
f_1 = \vect{v}^i \otimes \vect{w}^j \otimes \vect{u}^k \times \vect{z}_s^{i,j,k} \nonumber \\
\frac{\partial f_1}{\partial u_{1}^k} = \frac{\partial (u^k_1v^i_1w^j_1z_{1,1,1}+u^k_1v^i_1w^j_2z_{1,1,2}+u^k_1v^i_2w^j_1z_{1,2,1}+u^k_1v^i_2w^j_2z_{1,2,2})} {\partial u_{1}^k} \nonumber \\
= v^i_1w^j_1z_{1,1,1}+v^i_1w^j_2z_{1,1,2}+v^i_2w^j_1z_{1,2,1}+v^i_2w^j_2z_{1,2,2} \nonumber \\
= \vect{v}^i \otimes \vect{w}^j \times \tilde{\vect{z}} \nonumber \\
f_2 = \log{\sum\limits_{m,n,l} e^{v^i_m w^j_n u^k_l}}) \nonumber \\
\frac{\partial f_2}{\partial u_{1}^k} = \frac{1}{\sum\limits_{m,n,l} e^{v^i_m w^j_n u^k_l}}\frac{\partial \sum\limits_{m,n} e^{v^i_m w^j_n u^k_1}}{\partial u_{1}^k} \nonumber \\
=\frac{\sum\limits_{m,n} v^i_m w^j_n e^{v^i_m w^j_n u^k_1}}{\sum\limits_{m,n,l} e^{v^i_m w^j_n u^k_l}} \nonumber \\
=\sum\limits_{m,n} v^i_m w^j_n e^{v^i_m w^j_n u^k_1-\log{\sum\limits_{m,n,l} e^{v^i_m w^j_n u^k_l}}}
\end{align}
$\tilde{\vect{z}}$ only contains elements of $\vect{z}_s^{i,j,k}$ which will multiply $u_{1}^k$ in $\vect{v}^i \otimes \vect{w}^j \otimes \vect{u}^k$

\subsection{Update $\Sigma_u$}
Given $\vect{u}^{n,j_n}$, for $ j_n \in [1:J_n]$, $n\in [1:N]$, we can sample $\sigma_u^n$ from the posterior using:
\begin{align}
p(\sigma_u^n |\cdot) \propto \prod \limits_{j_n=1}^{J_n} \prod \limits_{i_n=1}^{I_n} p(u^{n,j_n}_{i_n}|\sigma_u^n)p(\sigma_u^n)
\end{align}
\subsection{Update $\Phi$}
 To reduce clutter, we abbreviate the subscript and superscript of $\vect{x}_m^{j_1,\dots,j_N}$ as $g = [m, (j_1,\dots,j_N)]$ and denote $\vect{x}_m^{j_1,\dots,j_N}$ as $\vect{x}_g$. Let use $\mathcal{G}^k_{i_1,\dots,i_N}$ to denote the set of $g$'s of $\vect{x}$'s which belong to cluster $k$ of basis measure $G^*_{i_1,\dots,i_N}$. Then we draw a new value for $\phi^k_{i_1,\dots,i_N}$ according to the following probability:
\begin{align}
p(\phi^k_{i_1,\dots,i_N}|\cdot) \propto \prod \limits_{g \in \mathcal{G}^k_{i_1,\dots,i_N}} f(\vect{x}_g |\phi^k_{i_1,\dots,i_N}) H(\phi^k_{i_1,\dots,i_N})
\end{align}
